# Supplementary material for: Diffusing Up the Hill: Dynamics and Equipartition in Highly Unstable Systems
Source: arXiv:1803.07833 ancillary file (2018-11-08)
Supplement: Supplementary file 1 [file SMx3.pdf]

# Supplemental Material
# Diffusing up the Hill: Dynamics and Equipartition in Highly Unstable Systems

Martin Šiler,[1,*] Luca Ornigotti,[2] Oto Brzobohatý,[1] Petr Jákl,[1]
Artem Ryabov,[3,†] Viktor Holubec,[3,4] Pavel Zemánek,[1] and Radim Filip[2]

[1] *Institute of Scientific Instruments of the Czech Academy of Sciences, Královopolská 147, 612 64 Brno, Czech Republic*
[2] *Department of Optics, Palacký University, 17. listopadu 1192/12, 771 46 Olomouc, Czech Republic*
[3] *Charles University, Faculty of Mathematics and Physics, Department of Macromolecular Physics, V Holešovičkách 2, 180 00 Praha 8, Czech Republic*
[4] *Universität Leipzig, Institut für Theoretische Physik, Postfach 100 920, D-04009 Leipzig, Germany*

(Dated: August 22, 2018)

## I. EXPERIMENTS

Contrary to our previous experimental work, where we measured short-time transient dynamics of moments and first passage times [1], here, we have used the experimental setup based on the counter-propagating light fields [2] in the configuration proposed theoretically in Ref. [3]. The proposal was tailored to elliminate systematic changes in the optical potential at a cost of the number of measured trajectories. By using this design we avoided the surface proximity effects, i.e. the fact that the immersion viscosity becomes anisotropic close to the surface [1]. Using the dual-beam setup we created two pairs of laser beams ($\lambda_{\rm vac} = 1064$ nm) having beam waist radius $w_0 = 4\ \mu$m. The propagation axes of both beams were separated by a distance 7.8 $\mu$m and the ratio of laser beam intensities was 0.48 in both beams. The beams were carefully adjusted to produce unstable potentials (see Fig. S1) with high precision. The sample consisted of polystyrene spheres of diameter 1 $\mu$m (Bangs Laboratories) diluted in water and sealed in a glass rectangular cuvette.

Firstly, single particle was trapped in an initial position by a single pair of laser beams. Then, using the spatial light modulator, the light field was reconfigured and the motion of the particle was recorder by a CCD camera (Basler Ace) at 2000 fps. After traveling through the highly unstable potentials, the particle was transported back to the initial location. Fig. 1 in the main text presents an example of recorded trajectories for the cubic potential. Using these trajectories we reconstructed the profile of optical force using the kernel smoothing algorithm [4] and integrated it to get the potential, presented as the dotted curve in top panel of Fig. 1 and by crosses in Fig. S1.

In total $\approx 100$ trajectories were recorded this way for a given potential under the same experimental conditions. Higher number of trajectories was not practically reachable because of high instability of studied potentials. After $\approx 100$ trajectories a readjustment of the experimental system was needed to compensate intrinsic mechanical drifts, which varied the nonlinear potential profile. This can cause a systematic changes which we avoided by the readjustment. Thus the new set of trajectories could not be mixed with the previous one into larger statistical ensemble. This limitation is generic for highly unstable potentials. The number of non-divergent trajectories diffusing around the origin reduces faster for higher instability, see Fig. S1 where the number of samples for $x_{\rm max}(t)$ and $\sigma(t)$ reduce faster in time for stronger instability.

In addition to the cubic potential from the main text, Fig. S1 shows further experimental results for all three typical basic classes of unstable potentials. On the left is the cubic potential with the shape exhibiting an inflection point at $x = 0$. In the middle, a less unstable potential than the cubic one is shown, with a meta-stable local minimum, . On the right, we present a more unstable potential than the cubic with neither a minimum nor an inflection point, . For all potentials we observe a convergence towards the quasi-stationary PDF $Q_{\rm st}(x)$. Position of the PDF maximum $x_{\rm max}$ as well as the curvature evolve in accordance with theoretical predictions.

The right column of the Fig. S1 contains the most unstable potential of all measured: the unstable potential without a stationary point. Here, trajectories diverge extremely fast which can be seen in lower panels of the column, where curves for local quantities are terminated as soon as there are less than 10 trajectories. Large fluctuations observed in the local quantities are a direct consequence of small (decreasing) number of trajectories surviving up to a given time [see also Fig. S2]. This is a limitation of the proposed methodology. A significantly larger sample of trajectories would be needed to observe more details from the experiment, when the potential is more unstable. This conflicts with a high instability of the potential.

## II. RECONSTRUCTION OF $Q(x,t)$

We used the following procedure to reconstruct PDFs from the measured trajectories assuming that the particle is placed at preselected $x_0$ at time $t_0 = 0$ [1]:

* siler@isibrno.cz
† rjabov.a@gmail.com

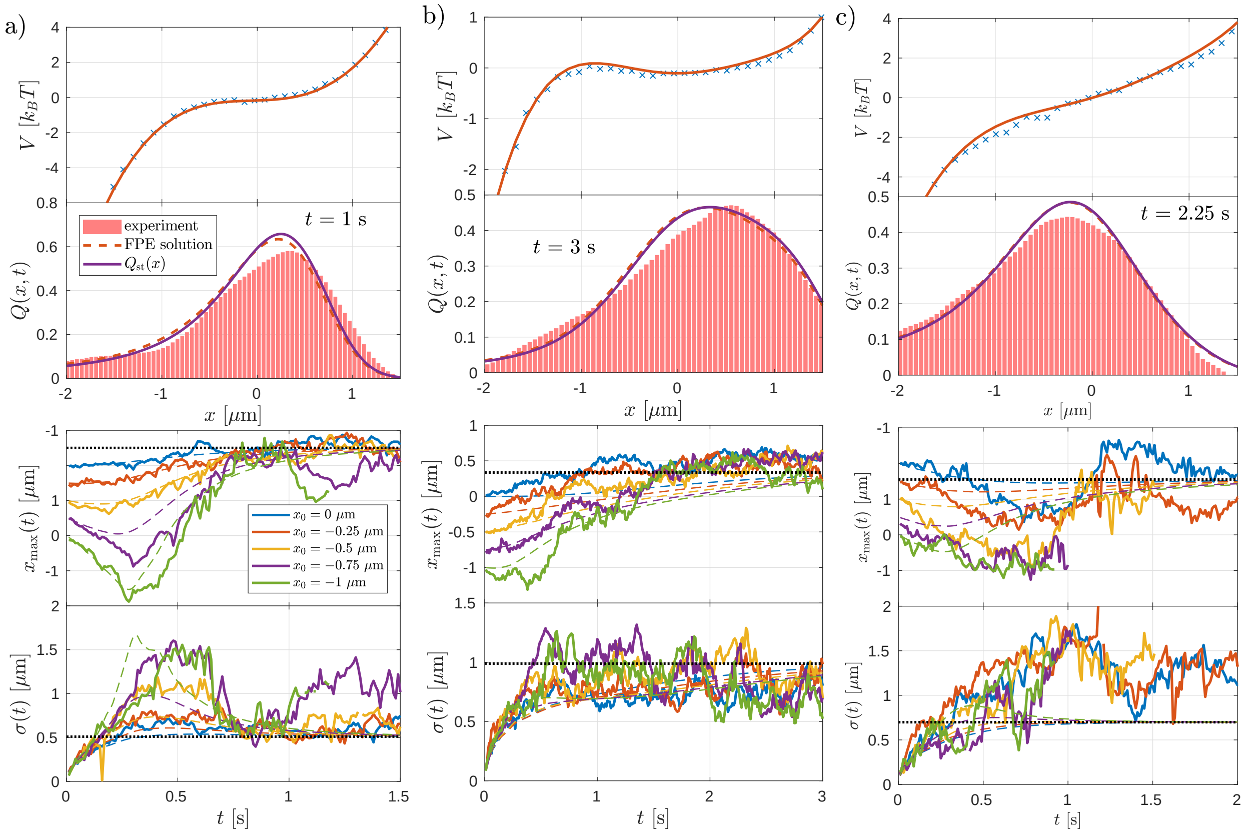


FIG. S1. Three generic examples of highly unstable potentials with different types of instability: The cubic potential with an inflection point at $x = 0$ [the left column a)], the potential with a meta-stable minimum [the middle column b)], and the unstable potential without a stationary point [the right column c)]. Upper panels: crosses represent experimentally determined potentials, the solid full lines show polynomial fits used in theory. The quasi-stationary PDF fits adequately experimental data despite a small sample of trajectories. For more stable potentials [the middle column b)], $x_{\max}(t)$ and $\sigma(t)$ converge well to theory. For more unstable potentials like [cf. the right column c)], the local quantities are affected by the quick reduction of number of non-diverging trajectories.

1. We take $i$-th trajectory out of $N$ recorded trajectories. We look for a point where the trajectory crosses $x_0$. This event corresponds to the initial point and the time is set to $t = 0$.

2. Following the same trajectory we move to the selected time $t$ and add the corresponding particle position into the ensemble.

3. Steps 1 and 2 are repeated for the subsequent unprocessed points of the same $i$-th trajectory. If there are no such new points in $i$-th trajectory satisfying conditions 1 or 2, we switch to $i+1$-th trajectory and repeat the steps 1-3.

This procedure generates a larger ensemble of independent data points corresponding to different $t$ compared to the number of recorded trajectories. Finally, the PDF at the time $t$ is recovered using the kernel smoothing algorithm. Because an analytical formula for the PDF satisfying Eq. (S3) is not known explicitly, the fit of the experimental statistics is a challenging problem, especially, for small number of trajectories. In order to obtain the position of the PDF mode (and its curvature) we used a parametrization of the experimental PDF based on the skewed normal distribution [5] in the form

$$P(x,t) = A\exp\left\{-\frac{(x-B)^2}{2C^2}\right\}\left(1+\mathrm{erf}\left[D\frac{(x-B)^2}{2C^2}\right]\right)+E \qquad \text{(S1)}$$

where $A \ldots E$ are the fitted parameters. We choose this profile as it allows us to parameterize the experimental PDF over an extended coordinate range while keeping the most prominent features of the PDF, namely its asymmetric skewed decrease. This parametrization of the fit is not unique, of course. Many of skewed distributions can be considered for the fitting. For instance, one may consider a parameterization taking into account only several terms of a polynomial expansion close to the maximum but in such a case the obtained position of PDF maximum and its curvature would be strongly influenced by the local noise of the reconstructed PDF profile. Eq. (S1), however, provides a reasonable compromise that enables to parameterize the experimental PDF keeping the number of fitted parameters minimal.

## III. ZERO-NOISE LIMIT

The transient atypical shift of $x_{\max}(t)$ against the acting force and the transient dynamics of the local standard deviation $\sigma(t)$ can be observed down to the limit of zero thermal noise ($T \to 0$), where PDF becomes [6, 7]

$$Q(x,t) = \theta\left(\frac{1}{\kappa t} - x\right) \frac{\exp\left\{-\frac{1}{2\sigma_0^2}\left(\frac{x}{1-\kappa x t} - x_0\right)^2\right\}}{S(t)\sqrt{2\pi\sigma_0^2}(1-\kappa x t)^2}, \tag{S2}$$

assuming Gaussian distribution with the mean $x_0$ and variance $\sigma_0^2$ at $t = 0$. Above, $\kappa = \mu/\gamma$ is the scaled potential strength, $S(t)$ is the so called survival probability [8] which gives the relative weight of nondivergent trajectories, $S(t) = \left[1 + \mathrm{erf}\left(\frac{1+\kappa x_0 t}{\sqrt{2\sigma_0^2}\kappa t}\right)\right]/2$, and $\mathrm{erf}(\bullet)$ is the error function. The Heaviside step function $\theta(\bullet)$ truncates the PDF creating the "light tail", i.e. the depleted region with zero occupation probability, $Q(x,t) = 0$ for $x > 1/\kappa t$. This tail, however, is not observable at the temperature of experiment, see Fig. S1. For long times, both $x_{\max}(t)$ and $\sigma(t)$ vanish, which reflects the behavior of trajectories stopping at the infection point. The trajectories cannot pass $x = 0$ without the thermal noise. The quasi-stationary $x_{\max} > 0$ reported in the main text is a thermally induced effect.

The zero-noise limit predicts the turning point of $x_{\max}(t)$ observed for large negative $x_0$, see lower panels in Fig. S1. However, it is challenging to give a quantitative agreement of the theory for cubic dynamics with the experiment. The perturbative extension of the theory for a weak thermal noise [7] deviates from the exact dynamics after a very short time. Hence even a weak noise has a pronounced effect on the dynamics of highly unstable systems. In the example of the cubic potential, the noise redistributes particles by almost free Brownian motion on the potential plateau, defined approximately as a region where $|V(x)|/k_BT < 1$. The nonperturbative treatment of the noise is indispensable for a correct prediction of the position PDF for intermediate and longer times.

## IV. EXPONENTIAL DECREASE IN NUMBER OF OBSERVED TRAJECTORIES FOR DIFFERENT INITIAL CONDITIONS

The Fokker-Planck equation, which determines the time-evolution of the particle position PDF in the potential $V(x)$, is given by

$$\partial_t P(x,t) = \frac{1}{\gamma}\left[k_BT\partial_{xx}^2 + \partial_x V'(x)\right] P(x,t). \tag{S3}$$

For a stable dynamics (confining potential $V(x)$), $P(x,t)$ converges in the long-time limit towards the Gibbs equilibrium PDF, $P_{\mathrm{eq}}(x) \sim \exp[-V(x)/k_BT]$. On the other hand, unstable systems (with non-confining potentials) possess no long-time equilibrium state. In the cubic potential, the fast decay of the initial state leads to a decay of normalization of the PDF $P(x,t)$ [7]. It is caused by rapidly diverging trajectories which reach $x = -\infty$ in a finite time.

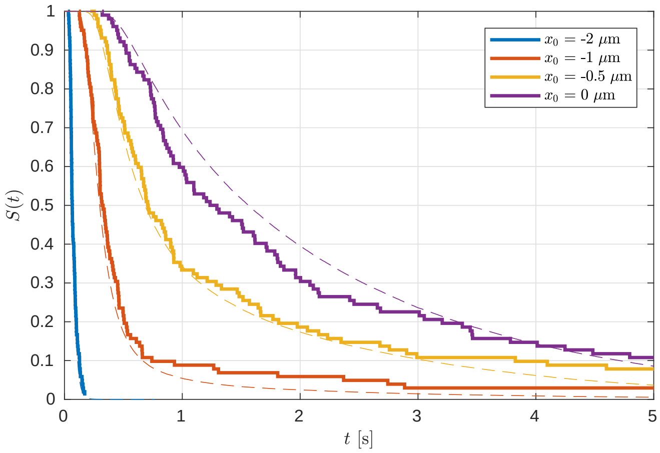


FIG. S2. Measured survival probability $S(t)$ (solid lines) starting at different initial positions $x_0$ for the cubic potential discussed in the main text. The dotted lines show results of numerical simulations. The figure demonstrates how the strong instability of the potential practically limits the duration of experiments for a fixed number of trajectories. The relative size of the ensemble of non-diverging trajectories [equal to $S(t)$] processed into the measured PDFs decreases exponentially for longer times. For both the large negative $x_0$, $x_0 < -1$ $\mu$m, and the long times, $t > 3$ s, it is practically impossible to get a reasonable statistics from a limited dataset of $\approx 100$ trajectories.

The norm of $P(x,t)$,

$$S(t) = \int_{-\infty}^{+\infty} dx P(x,t), \tag{S4}$$

known also as the survival probability [8], gives the relative weight of trajectories that have not reached $x = -\infty$ by the time $t$. For nonzero thermal noise ($T > 0$), the survival probability decays exponentially with time, $S(t) \sim s_0 \mathrm{e}^{-\lambda_0 t}$. Thus, the total weight of trajectories wandering near the inflection plateau decreases as the individual trajectories are quickly dragged towards minus infinity.

To demonstrate one of the most challenging aspects of the experiment, we have investigated time before divergence in the experimental potential and the number of trajectories which contribute to the quasi-stationary PDF when the initial position $x_0$ varies. The measured survival probability $S(t)$ for the particle initially placed in various negative starting positions $x_0$ (solid staircase lines) and the results of numerical Monte-Carlo simulations (dashed lines) are plotted in Fig. S2 for the ideal cubic potential with stiffness 4.07 $k_BT\mu\mathrm{m}^{-3}$ from the main text. In simulations we generated $10^8$ trajectories staring

from the given location $-2 \leq x_0 \leq 0$ $\mu$m. A trajectory was classified as divergent when it crossed $x = -10$ $\mu$m.

For all $x_0$ we initially observe a plateau of $S(t) \approx 1$ followed by an exponential decay. For initial positions $x_0 \ll -1$ $\mu$m, the survival probability almost immediately approaches zero. However, for $x_0 \approx -1$ $\mu$m (where the potential is already two times larger than $k_B T$), we start to observe a sufficient number of non-diverging trajectories even for times $t > 1$s, which is enough for all experimental demonstrations.

## V. QUASI-STATIONARY DISTRIBUTION

Even though there exists no equilibrium distribution in non-confining potentials, there may exist a quasi-stationary state with a constant spatial profile of the PDF. Exact meaning and emergence of the quasi-stationary state is best seen when we write the solution of Eq. (S3) as the eigenvalue expansion [9]

$$P(x,t) = \sum_{n=0}^{\infty} \psi_n(x) \mathrm{e}^{-\lambda_n t}, \tag{S5}$$

where $\psi_n(x)$ are eigenvectors of the Fokker-Planck operator satisfying

$$\frac{1}{\gamma} \left[ k_B T \partial^2_{xx} + \partial_x V'(x) \right] \psi_n(x) = -\lambda_n \psi_n(x). \tag{S6}$$

The survival probability is then given by

$$S(t) = \sum_{n=0}^{\infty} s_n \mathrm{e}^{-\lambda_n t}, \tag{S7}$$

with $s_n = \int_{-\infty}^{+\infty} dx \psi_n(x)$.

The sub-ensemble of trajectories which survive up to time $t$ is described by the conditional PDF

$$Q(x,t) = \frac{P(x,t)}{S(t)}. \tag{S8}$$

If $t$ is large, the PDF $Q(x,t)$ describes statistics of long-living trajectories. If $P(x,t)$ decays exponentially in time as in Eq. (S5) (this is exactly what we define as the “highly unstable system”), the conditional PDF $Q(x,t)$ converges to the time-independent quasi-stationary PDF $Q_{\mathrm{st}}(x)$, i.e.,

$$Q_{\mathrm{st}}(x) = \lim_{t\to\infty} Q(x,t). \tag{S9}$$

The convergence towards the quasi-stationary limit, which is very fast in our experiment, is justified after we introduce expansions (S5) and (S7) into the definition (S8). For large $t$, this yields

$$Q(x,t) \approx Q_{\mathrm{st}}(x) + Q_1(x) \mathrm{e}^{-(\lambda_0-\lambda_1)t} + \ldots \tag{S10}$$

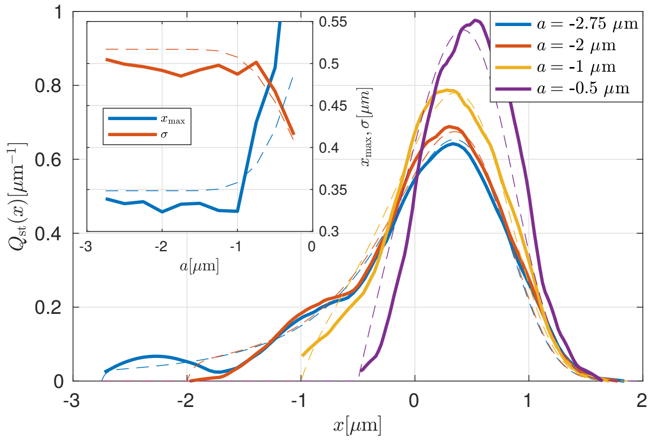


FIG. S3. Measured PDFs at the time $t = 1.15$ s (solid) compared with the theoretical quasi-stationary PDFs $Q_{\mathrm{st}}(x)$ computed from Eq. (4) from the main text (dashed) for three different positions of the absorbing boundary $a$. The inset shows experimental (solid) and theoretical (dashed) values of $x_{\max}$ and $\sigma$ as the functions of $a$. For $a \ll 0$ the quantities become $a$-independent.

with $Q_{\mathrm{st}}(x) = \psi_0(x)/s_0$ and the exponentially-decaying correction factor $Q_1(x) = Q_{\mathrm{st}}(x)[\psi_1(x) - s_1]$. The quasi-stationary PDF is given by the normalized eigenvector corresponding to the smallest (in the absolute value) eigenvalue $\lambda_0$. This justifies that the quasi-stationary PDF can be computed from the quasi-stationary Fokker-Planck equation (4) from the main text. Alternatively, this equation can be obtained after we introduce the asymptotic approximation $P(x,t) \sim S(t) Q_{\mathrm{st}}(x) \mathrm{e}^{-\lambda_0 t}$ into the Fokker-Planck equation (S3). For a rigorous mathematical approach to the theory of quasi-stationary distributions we refer to the book [10].

In order to solve the eigenvalue problem (S6) for the quasi-stationary distribution:

$$\frac{1}{\gamma} \left[ k_B T \partial^2_{xx} + \partial_x V'(x) \right] Q_{\mathrm{st}}(x) = -\lambda_0 Q_{\mathrm{st}}(x), \tag{S11}$$

we need to specify boundary conditions. The integrability of $Q_{\mathrm{st}}(x)$ requires that $\lim_{|x|\to\infty} Q_{\mathrm{st}}(x) = 0$. The potential is confining for $x \to +\infty$, which implies that also the probability current [9] vanishes for large positive $x$. Contrary to this, the instability at $x = -\infty$ acts as a natural sink. Even though the PDF vanishes there, the current is non-zero in the limit $x \to -\infty$ [7].

Of course, the limit $|x| \to \infty$ is nothing but mathematical idealization. Both in the numerical solution of Eq. (4) from the main text and in the experiment we always work within a finite bounded region. To reproduce properly the PDF defined on the infinite interval $x \in (-\infty, +\infty)$, we impose the following boundary conditions. The right boundary $x = b$, $b > 0$ is reflecting (both the probability and the current vanishes at the boundary). If we choose $b$ large enough such that the thermal energy is not sufficient to reach $x = b$ in a reasonably short time, i.e., $b \gg (3k_B T/\mu)^{1/3}$, the finite $b$ will well approximate

$b = \infty$. The left boundary, $x = a$, $a < 0$ is absorbing, i.e., $Q_{\rm st}(a) = 0$. Again, when $a \ll -(3k_BT/\mu)$, we obtain a reasonable approximation of the PDF for $a = -\infty$. Fig. S3 shows the PDF for various positions of the absorbing boundary $a$, $a < 0$. The inset shows the PDF maxima and the curvature. Here, we can see that for $a \lesssim -1.5$ $\mu$m we obtain a good correspondence of the experimental PDF and the predicted $Q_{\rm st}(x)$ for $a = -\infty$. On the contrary, for absorbing boundary closer to the inflection point, we see that especially the position of PDF maximum deviates.

Notice, that the quasi-stationary distribution $Q_{\rm st}(x)$ is independent of the initial distribution at $t = 0$, $Q(x, 0) = P(x, 0)$. This fact is obvious, because the eigenvalue problem (S11) contains no trace of the initial state. In the limiting procedure $t \to \infty$, during which the quasi-stationary state is established, the information about the initial condition is contained in exponentially damped terms of the series (S10). Thus the dependence on the initial particle position PDF is lost exponentially fast.

## VI. SCALING ANALYSIS OF THE QUASI-STATIONARY FOKKER-PLANCK EQUATION

For the cubic potential in particular and for all unstable monomial potentials $V(x) = \mu x^n/n$, $n = 1, 3, 5$, the Langevin equation and the Fokker-Planck equation can be brought into the dimensionless form by a proper coupling of the space and time scales. The scaling is not very useful for the analytical solution of the equations. Its actual power is to show how quantities associated with length (time) depend on the ambient temperature. For instance, in the quasi-stationary state the scaling predicts that the local quantities scale as

$$x_{\rm max} \sim (k_BT/\mu)^{1/3}, \quad \sigma \sim (k_BT/\mu)^{1/3}, \qquad \text{(S12)}$$

for $n = 3$, and for the decay rate, which has units 1/s, we obtain

$$\lambda_0 \sim \frac{\mu}{\gamma}\left(\frac{k_BT}{\mu}\right)^{1/3}, \qquad \text{(S13)}$$

where the temperature can be also hidden in the friction coefficient $\gamma$, $\gamma = \gamma(T)$.

To see this, we define the thermal length scale $l$ and the time scale $s$,

$$l = \left(\frac{k_BT}{\mu}\right)^{1/n}, \qquad s = \frac{\gamma}{\mu}\left(\frac{\mu}{k_BT}\right)^{1-2/n}, \qquad \text{(S14)}$$

in such a way that the usual diffusive scaling is obeyed:

$$l^2 = Ds, \qquad D = \frac{k_BT}{\gamma}. \qquad \text{(S15)}$$

The scaled dimensionless variables defined as

$$\chi(t) = x(t)/l, \qquad \tau = t/s, \qquad \text{(S16)}$$

measure the space and the time in units of $l$ and $s$, respectively.

The Langevin equation [Eq. (1) in the main text] expressed in coordinates (S16) reads

$$\frac{d\chi}{d\tau} = -\chi^{n-1} + \sqrt{2}\,\xi. \qquad \text{(S17)}$$

The corresponding Fokker-Planck equation (S3) becomes

$$\partial_\tau f(\chi, \tau) = \left[\partial^2_{\chi\chi} + \partial_\chi \chi^{n-1}\right] f(\chi, \tau). \qquad \text{(S18)}$$

The both equations are now dimensionless and independent of the parameters $T$, $\gamma$, and $\mu$.

Focusing on the quasi-stationary state, the dimensionless form of the quasi-stationary Fokker-Planck equation (S11) [Eq. (3) in the main text] reads

$$\left[\partial^2_{\chi\chi} + \partial_\chi \chi^{n-1}\right] f_{\rm st}(\chi) = -\theta_0 f_{\rm st}(\chi). \qquad \text{(S19)}$$

where $\theta_0$,

$$\theta_0 = \lambda_0 s, \qquad \text{(S20)}$$

stands for the dimensionless decay rate. The solution $f_{\rm st}(\chi)$ is obviously independent of the parameters $T$, $\gamma$, and $\mu$. They enter the problem only through the scaling factors in the transformation to SI units:

$$Q_{\rm st}(x) = \frac{1}{l} f_{\rm st}(x/l). \qquad \text{(S21)}$$

Therefore, all quantities with the dimension of length ($x_{\rm max}$, $\sigma$) behave with temperature simply as $l$, and at the same time, the decay rate $\lambda_0$ is proportional to $1/s$, hence Eqs. (S12) and (S13) for $n = 3$.

Last but not least, we note that the above discussion holds provided we have natural boundary conditions in $\pm\infty$. Otherwise, e.g., imposing the absorbing boundary at some $x = a$ introduces new additional length scale $a$, which may modify the predicted behavior Eqs. (S12) and (S13). However, based on the discussion in the last paragraph of Sec. V, see also Fig. S3, that the boundary does not influences results when its far enough from the plateau, we can expect that also the scaling will hold for a finite system with boundaries placed far from the origin.

## VII. GENERALIZED EQUIPARTITION THEOREM

The principle of energy equipartition is one of the most illuminating results of the kinetic theory and the classical statistical mechanics. Deviations from this principle stimulated further generalizations of the statistical mechanics to relativistic and quantum systems [11]. The principle was first formulated for degrees of freedom, which contribute by quadratic terms to the particle total energy. The generalized version of the principle was derived by Tolman [12] and became a standard textbook

topic known as "the equipartition theorem", see e.g. [13]. In the present notation, the theorem reads

$$\langle xV'(x)\rangle_{\rm eq} = k_B T, \tag{S22}$$

where the average is taken over the equilibrium Gibbs distribution.

The Gibbs equilibrium distribution emerges in the long-time limit in a stable system in contact with the heat bath. The most straightforward way how to stabilize the particle in the cubic potential is to bound its motion to the stable region $x > 0$ of the potential. This can be accomplished by placing an infinite potential wall (or the so called reflecting boundary) at the origin. Then, the Gibbs equilibrium state becomes $Q_{\rm eq}(x) = \theta(x)\exp[-V(x)/k_BT]/Z$, where $\theta(x)$ is the Heaviside function due to the potential wall and $Z$ stands for the partition function of the semi-infinite system, $Z = \int_0^{+\infty} dx \exp[-V(x)/k_BT]$.

The average energy of the particle is one of the principle quantities in stochastic and classical thermodynamics [11, 14, 15]. For the stabilized potential formed by a simple monomial, $V(x) \sim x^n$ for $x > 0$, the theorem (S22) yields the mean potential energy in the form

$$\langle V(x)\rangle_{\rm eq,+} = \frac{k_BT}{n}. \tag{S23}$$

Let us now show that the equipartition theorem can be generalized to the case of quasi-stationary states. Using this generalization, we derive the mean energy of the particle in the unstable potential and show that it is always higher than (S23).

The quasi-stationary equipartition theorem stated in the main text, cf. Eq. (6),

$$\langle V(x)\rangle_{\rm st,+} = \frac{k_BT}{n} + \frac{\lambda_0\gamma}{2n}\left\langle x^2\right\rangle_{\rm st,+}, \tag{S24}$$

is a special case of the more general principle,

$$\langle xV'(x)\rangle_{\rm st,+} = k_BT + \frac{\lambda_0\gamma}{2}\left\langle x^2\right\rangle_{\rm st,+}. \tag{S25}$$

Eq. (S25) reduces to Eq. (S24) when the potential is given by a simple monomial, $V(x) \sim x^n$. In the both equations (S24) and (S25), the average is performed over the normalized, sufficiently stable, part of the quasi-stationary PDF based on the positive half-line $x > 0$, i.e., over

$$Q_{\rm st,+}(x) = \frac{\theta(x)Q_{\rm st}(x)}{\int_0^\infty dx' Q_{\rm st}(x')}. \tag{S26}$$

Notice that $\lambda_0 = 0$ corresponds to the stable potential. In this case, the conditional PDF (S26) is nothing but the Gibbs equilibrium in the stable semi-infinite system, $Q_{\rm eq}(x) = \theta(x)\exp[-V(x)/k_BT]/Z$, and Eqs. (S25) and (S24) reduce to Eqs. (S22) and (S23), respectively.

In the unstable case, $\lambda_0 > 0$, there is no equilibrium PDF. Instead, the quasi-stationary state emerges at longer times. The PDF (S26) is a conditional quasi-stationary PDF conditioned on the event that the particle is located on a positive half-line. From the experimental point of view, the mean energy (S24) can be measured using the following post-selection process. First, the particle evolves for a reasonably long time such that the quasi-stationary state emerges. After that, we measure the position of the particle. If it is negative, we discard the measurement and repeat the experiment. If the position is positive, we compute and record the particle potential energy. Average over many such experiments yields the mean energy given by Eq. (S24).

Eq. (S25) can be derived for any potential $V(x)$, which is confining for $x > 0$. That is, the potential grows fast with increasing $x$ such that the probability current vanishes in the limit $x \to \infty$. Formally, we obtain Eq. (S25) from the quasi-stationary Fokker-Planck equation (S11) [also Eq. (3) in the main text] after multiplication by $x^2$ and integration over the positive half line $x \in (0, \infty)$:

$$\frac{2k_BT}{\gamma}\int_0^\infty dx\, Q_{\rm st}(x) - \frac{2}{\gamma}\int_0^\infty dx\, xV'(x)Q_{\rm st}(x) = -\lambda_0\int_0^\infty dx\, x^2 Q_{\rm st}(x). \tag{S27}$$

To obtain this equation, we have further used integration per partes with the assumption that the PDF and its first derivative vanishes sufficiently fast as $x \to \infty$, which is a reasonable assumption for the right-confining potential $V(x)$. Dividing Eq. (S27) by the normalization factor, $\int_0^\infty dx\, Q_{\rm st}(x)$, appearing in the first term on the left-hand side, we recognize that other terms are nothing but averages over the normalized PDF $Q_{\rm st,+}(x)$ from Eq. (S26). This way we obtain

$$\frac{2k_BT}{\gamma} - \frac{2}{\gamma}\langle xV'(x)\rangle_{\rm st,+} = -\lambda_0\left\langle x^2\right\rangle_{\rm st,+}, \tag{S28}$$

which, after straightforward algebraic manipulations, leads to Eq. (S25).

Moreover, for the cubic potential, the behavior of principal characteristics with temperature is given by $x_{\max} \sim (k_BT/\mu)^{1/3}$, $\sigma \sim (k_BT/\mu)^{1/3}$, and $\lambda_0 \sim (\mu/\gamma)\,(k_BT/\mu)^{1/3}$, see the previous section. The scaling implies that the excess energy in Eq. (S24) behaves as $\lambda_0\left\langle x^2\right\rangle_{\rm st,+} \sim k_BT/\mu$. Hence the difference between the quasi-stationary and the equilibrium equipartition theorems increases with $T$.

[1] M. Šiler, P. Jákl, O. Brzobohatý, A. Ryabov, R. Filip, and P. Zemánek, Sci. Rep. **7**, 1697 (2017).
[2] T. Čižmár, O. Brzobohatý, K. Dholakia, and P. Zemánek, Laser Phys. Lett. **8**, 50 (2011).
[3] P. Zemánek, M. Šiler, O. Brzobohatý, P. Jákl, and R. Filip, J. Opt. **18**, 065402 (2016).
[4] D. Lamouroux and K. Lehnertz, Physics Letters A **373**, 3507 (2009).
[5] A. O'Hagan and T. Leonard, Biometrika **63**, 201 (1976).
[6] R. Filip and P. Zemánek, J. Opt. **18**, 065401 (2016).
[7] L. Ornigotti, A. Ryabov, V. Holubec, and R. Filip, Phys. Rev. E **97**, 032127 (2018).
[8] S. Redner, *A guide to first-passage processes*, 1st ed. (Cambridge University Press, 2007).
[9] H. Risken, *The Fokker-Planck Equation: Methods of Solutions and Applications*, 2nd ed., Springer Series in Synergetics (Springer, 1996).
[10] P. Collet, S. Martínez, and J. San Martín, *Quasi-Stationary Distributions: Markov Chains, Diffusions and Dynamical Systems* (Springer-Verlag Berlin Heidelberg, 2013).
[11] R. C. Tolman, *The Principles of Statistical Mechanics* (Clarendon Press, 1938).
[12] R. C. Tolman, Phys. Rev. **11**, 261 (1918).
[13] K. Huang, *Statistical Mechanics*, 2nd ed. (Wiley, 1987) Chap. 6.4.
[14] K. Sekimoto, *Stochastic Energetics* (Springer, Heidelberg, 2010).
[15] U. Seifert, Rep. Prog. Phys. **75**, 126001 (2012).
